# Supplementary material for: FloMore: Meeting bandwidth requirements of flows
Source: arXiv:2108.03221 source file (2021-08-06)
Supplement: Supplementary file 1 [file zappendix.tex]

\subsection{More information on hint example (for internal purpose)}
\textbf{Why \FFCimp{} achieves 2/3?}
Let rs1T be reservation on the tunnels s-1-T, and use similar
notation for other tunnels. Then, since the reservation must be met on any two link failures, it should be met when 1-T, and 2-T are down. Then, 
reservation is at most $rs3T + rs43T = 0.5 + rs43T$, since rs3T cannot exceed 0.5 which is the capacity of the link s-3. Likewise, the reservation is at most $0.5 + rs42T$, and $0.5 + rs41T$. Thus the total reservation cannot exceed more than $0.5 + min(rs41T,rs42T, rs43T) = 0.5 + 0.5/3$, since $rs41T + rs42T + rs43T \leq 0.5$

\textbf{What does \LS{} achieves?}
Let the LS be s-4-T with reservation $b$.
The s-t reservation is carried by the 6 s-T tunnels, and $b$.
This must be met under any 2 failure scenario. Since it must be met 
when 1-T and 2-T fail, we have the reservation is at most rs3T + rs43T + b.
Similarly, the reservation is at most rs1T+rs41T+b, and at most rs2T + rs42T + b.

Next the logical segment s-4 must carry b across all 2 failures.
The tunnels are s-1-4,s-2-4,s-3-4, s-4, with reservations rs14 etc.
Consider where s-1 and s-2 fail. Then, rs34 + rs4 >= b.

Combining with the above, the total s-t reservation is at most
rs3T + rs43T + rs34 + rs4.

Now rs3T + rs34 is the total reservation of all tunnels that traverse
s-3, and hence this sum is bounded by 0.5.

So, the s-t reservation is at most 0.5 + rs4 + rs43T.
By a similar set of arguments, the s-t reservation is at most
0.5 + rs4 + rs42T, and 0,5 + rs4 + rs41T. Hence, it is at most
0.5 + rs4 + min(rs43T,rs42T,rs41T).

Now, take the capacity constraint of link s-4.
rs4 + rs43T + rs42T + rs41T = 0.5.
Hence, rs43T+rs42T+rs41T = 0.5-rs4, and min(rs43T,rs42T,rs41T) = (0.5-rs4)/3

Then, s-t reservation is at most 0.5 + rs4 + (0.5-rs4)/3,
which works out to 2/3 + 2/3 * rs4.

\textbf{Alternate argument to give upper bound on objective with logical sequence, no hint.}

Let b be the reservation on the logical sequence s-4-T.
Then, b must be guaranteed on s-4 under two failures,
and on 4-T under two failures.

Consider the segment 4-T. We have 
$r41T+r42T+r43T \geq b$ under any two failures. 
Consider failure of 4-1 and 4-2. Then, $r43T \geq b$. 
Now consider capacity constraint of link 4-3.
$rs43T + r43T <= 0.5$. Hence, $rs43T \leq 0.5 - r43T \leq
0.5 -b$. Similar constraints for $rs42T$, and $rs41T$.

Next consider the segment s-4. We have 
$rs4 + rs14 + rs24 + rs34 \geq b$ under any two failures.
Consider failure of s-4 and s-1. Then,
$rs24 + rs34 \geq b$. We get two similar constraints
by failing s4 and each of s-2, s-3, and sum these constraints.
We get $2(rs14+rs24+rs34) \geq 3b$. Denote rs14+rs24+rs34 as R.
Then, $R \geq 3b/2$.

Now consider the total reservation from s-t.
This is $b + rs1T + rs2T + rs3T + rs41T + rs42T + rs43T$,
which must be upheld under any two failures. Consider the failure 
of links 1-T, and 2-T. Then, the reservation is at most
$b + rs3T + rs43T$. We get similar bounds on reservation by
failing pairs of links 1-T, 2-T and 3-T. Summing these,
we get reservation is at most 
b + (rs1T+rs2T+rs3T)/3 + (rs43T + rs42T +rs41T)/3

But, the numerator of the second term is at most 1.5 - R.
Combined with the cnstraints on rs43T etc. from above,
we get reservation is at most:

$\leq b + (1.5 - R)/3 + (1.5-3b)/3$ \\
$\leq b + 0.5 - R/3 + 0.5 - b$ \\
$\leq  1 - R/3$\\
$\leq 1 - b/2$ \\
$b$ can be at most 0.5, so, the bound is at most $3/4$.

\textbf{Proof of Proposition \ref{prop:linear_system}.} 
We will show $M \in \mathbb{R}^{P \times P}$ is invertible by showing $M$ is a weakly-chained diagonally dominant matrix, which is proven to be non-singular\cite{wcdd_math}. 

In a particular scenario $x$, let $T_x(s,t)$ denote the set of alive tunnels from $s$ to $t$, $L_x(s,t)$ denote the set of active \LS{}s from $s$ to $t$ and $\tau_x(s,t)$ denote the active \LS{}s which go through segment $(s,t)$. We first give the formal definition of $P$, the set of node pairs of interest. A node pair $(i_1,j_1) \in P$ if and only if there is a sequence of node pairs $(i_1,j_1)$, $(i_2,j_2)$,\ldots,$(i_k,j_k)$, such that $z_{i_kj_k}d_{i_kj_k}>0$ and $\forall m: 1 \le m \le k-1$, $\exists q \in L_x(i_{m+1},j_{m+1}) \cap \tau_x(i_m,j_m): b_q > 0$. That is to say a node pair $(i,j) \in P$ if and only if through several levels of \LS{}s, it can be useful to route some demand. Note that even though $P$ is a subset of all node pairs, the integrity of used \LS{}s is not violated on $P$, i.e., $\forall q: b_q > 0, q\in L_x(i_1,j_1), (i_1,j_1) \in P$, all of $q$'s underlying hops are also in $P$. Because if $(i_1,j_1) \in P$, there must be a sequence of node pairs $(i_1,j_1)$, $(i_2,j_2)$,\ldots,$(i_k,j_k)$ which satisfies the definition of $P$. If we also have $b_q > 0, q \in L_x(i_1,j_1)$, and $q \in \tau_x(i_0,j_0)$, it is clear that the sequence $(i_0,j_0), (i_1,j_1)$, $(i_2,j_2)$,\ldots,$(i_k,j_k)$ also satisfies the definition of P, hence $(i_0,j_0) \in P$.

Next, we formally define each entry in $M$. The diagonal of $M$ is the sum of available reservations on the pair, i.e. $\forall (i,j) \in P, M_{ij, ij} = \sum_{l \in T_x(i,j)} a_{l} + \sum_{q \in L_x(i,j)}b_{q}$. And other entries of $M$ denote how much a node pair needs to carry for other node pairs, i.e. $M_{ij, mn} = -\sum_{q \in \tau_x(i,j) \cap L_x(m,n)} b_{q}$ if $(i,j) \ne (m,n)$.

For each row $(i,j) \in P$, we sum over all entries in that row to get $\sum_{(m,n)\in P}M_{ij,mn} = \sum_{l \in T_x(i,j)} a_{l} + \sum_{q \in L_x(i,j)}b_{q} -\sum_{q \in \tau_x(i,j)} b_{q} \ge z_{ij}d_{ij} \ge 0$. The first inequality is given by the capacity constraint in our model. Thus, $M$ is a weakly diagonally dominant matrix.

From our definition of $P$, we know that $\forall (i_1,j_1) \in P$, there is a sequence $(i_1,j_1)$, $(i_2,j_2)$,\ldots,$(i_k,j_k)$, such that $z_{i_kj_k}d_{i_kj_k}>0$ and $\forall m: 1 \le m \le k-1$, $\exists q \in L_x(i_{m+1},j_{m+1}) \cap \tau_{i_m,j_m}: b_q > 0$. Thus, for each row $(i,j) \in P$, there is a sequence $(i_1,j_1)$, $(i_2,j_2)$,\ldots,$(i_k,j_k)$, such that $\sum_{(m,n)\in P}M_{i_kj_k,mn} = \sum_{l \in T_x(i_k,j_k)} a_{l} + \sum_{q \in L_x(i_k,j_k)}b_{q} -\sum_{q \in \tau_x(i_k,j_k)} b_{q} \ge z_{i_kj_k}d_{i_kj_k} > 0$, and $\forall m: 1 \le m \le k-1$, $M_{i_kj_k,i_{k+1}j_{k+1}} \ne 0$. This satisfies the definition of weakly-chained diagonally dominant matrix. So $M$ is a weakly-chained diagonally dominant matrix. Thus, $M$ is non-singular and there is always a unique solution $\vec{U^*}$ to the linear system $M \times \vec{U} = \vec{D}$.

Next, we use fixed-point theorem to prove that all entries of the solution are in $[0,1]$. Let $f(\vec{U})$ be a function mapping from $[0,1]^{P}$ to $\mathbb{R}^{P}$. And we define $f(\vec{U})$ as

\begin{align}
\begin{split}
& f(\vec{U})_{i,j} = \frac{\vec{D}(i,j) + \sum_{(m,n) \in P,q\in \tau(i,j)\cap L_x(m,n)}\vec{U}(m,n)b_q}{\sum_{l\in T_x(i,j)}a_l + \sum_{q\in L_x(i,j)}b_q} \\
\end{split}
\end{align}

It is easy to see that $\vec{U_0}$ is a solution to $M \times \vec{U} = \vec{D}$ if $f(\vec{U_0}) = \vec{U_0}$. With $\vec{U} \in [0,1]^{P}$, we have 

\begin{align}
\begin{split}
& f(\vec{U})_{i,j} \ge \frac{\vec{D}(i,j)}{\sum_{l\in T_x(i,j)}a_l + \sum_{q\in L_x(i,j)}b_q} \ge 0 \\
\end{split}
\end{align}

and 

\begin{align}
\begin{split}
& f(\vec{U})_{i,j} \le \frac{\vec{D}(i,j) + \sum_{(m,n) \in P, q\in \tau(i,j)\cap L_x(m,n)}b_q}{\sum_{l\in T_x(i,j)}a_l + \sum_{q\in L_x(i,j)}b_q} \le 1 \\
\end{split}
\end{align}

Since $f$ is a continuous function mapping from $[0,1]^{P}$ to $[0,1]^{P}$, and $[0,1]^{P}$ is a compact convex set, based on fixed-point theorem, we know that there is at least one point $U_0 \in [0,1]^{P}$ so that $f(U_0) = U_0$.
$\square$

\textbf{Proof of Proposition \ref{prop:valid_routing}} First, we need to show $r_{lt}$ satisfies the following flow balance constraint:

\begin{align}
\begin{split}
& ~~\sum_{j,l \in T_x(i,j)} r_{lt} - \sum_{j,l \in T_x(j,i)} r_{lt} 
= 
\begin{cases}
z_{it}d_{it} & i \ne t\\
-\sum_{j}z_{jt}d_{jt} & i = t
\end{cases}
\end{split}\label{eq:r_flow}
\end{align}

Based on the definition of $\vec{D_t}$ which contains all the traffic demand going to $t$, we have

\begin{align}
\begin{split}
& ~~\sum_{j} \vec{D_t}(i,j) - \sum_{j} \vec{D_t}(j,i)
= 
\begin{cases}
z_{it}d_{it} & i \ne t\\
-\sum_{j}z_{jt}d_{jt} & i = t
\end{cases}
\end{split}\label{eq:D_flow}
\end{align}

Since $M \times \vec{U^*_t} = \vec{D_t}$, we only need to prove 

\begin{align}
\begin{split}
& ~~\sum_{j,l \in T_x(i,j)} r_{lt} - \sum_{j,l \in T_x(j,i)} r_{lt} 
= \\
& ~~\sum_{j} (M\vec{U^*_t})(i,j) - \sum_{j} (M\vec{U^*_t})(j,i) \quad
\end{split}\label{eq:mu_flow}
\end{align}

$(M\vec{U^*_t})(i,j)$ contains all the reservations on physical tunnels and \LS{}s from $i$ to $j$, as well as the usage of $(i,j)$ for \LS{}s which contain it as a segment. We will show that in $(M\vec{U^*_t})(i,j) - \sum_{j} (M\vec{U^*_t})(j,i)$, the reservations and usage on \LS{}s will cancel out each other, leaving only the reservations on physical tunnels.

\begin{align}
\begin{split}
& ~~\sum_{j} (M\vec{U^*_t})(i,j) - \sum_{j} (M\vec{U^*_t})(j,i) = \\
& \sum_{j,l \in T_x(i,j)} a_{l}\vec{U^*_t}(i,j) - \sum_{j,l \in T_x(j,i)} a_{l}\vec{U^*_t}(j,i) + \\
& \sum_{j,q \in L_x(i,j)}b_{q}\vec{U^*_t}(i,j) - \sum_{j,q \in L_x(j,i)}b_{q}\vec{U^*_t}(j,i) + \\ 
& \sum_{j,q \in \tau_x(i,j)\cap L_x(m,n)} b_{q}\vec{U^*_t}(m,n) - \sum_{j,q \in \tau_x(j,i)\cap L_x(m,n)} b_{q}\vec{U^*_t}(m,n) 
\end{split}\label{eq:expland_mu_flow}
\end{align}

Now with any logical sequence $q \in L_x(s,t)$ being an integral sequence of segments from $s$ to $t$, we have the following properties:

$\bullet$ $\forall j,q\in L_x(i,j)$, suppose the first segment of $q$ is $(i,k)$, then $q \in \tau_x(i,k)\cap L_x(i,j)$. Similarly, $\forall j,q\in L_x(j,i)$, suppose the last segment of $q$ is $(k,i)$, then $q \in \tau_x(k,i)\cap L_x(j,i)$.

$\bullet$ $\forall j,q \in \tau_x(i,j)\cap L_x(m,n)$, if $i=m$, then $q \in L_x(i,n)$. Otherwise, $i$ is an intermediate node of the \LS{} $q$, suppose its predecessor is $k$, then $q \in \tau_x(k,i)\cap L_x(m,n)$. Similarly, $\forall j,q \in \tau_x(j,i)\cap L_x(m,n)$, if $i=n$, then $q \in L_x(m,i)$. Otherwise, $i$ is an intermediate node of the \LS{} $q$, suppose its successor is $k$, then $q \in \tau_x(i,k)\cap L_x(m,n)$.

From the above two properties, we know that for every $b_q$ term in \eqref{eq:expland_mu_flow}, there is a counter part in \eqref{eq:expland_mu_flow} which can cancel it, leaving only the $a_l$ terms in \eqref{eq:expland_mu_flow}, i.e.

\begin{align}
\begin{split}
& ~~\sum_{j} (M\vec{U^*_t})(i,j) - \sum_{j} (M\vec{U^*_t})(j,i) = \\
& \sum_{j,l \in T_x(i,j)} a_{l}\vec{U^*_t}(i,j) - \sum_{j,l \in T_x(j,i)} a_{l}\vec{U^*_t}(j,i) = \\
& ~~\sum_{j,l \in T_x(i,j)} r_{lt} - \sum_{j,l \in T_x(j,i)} r_{lt} 
\end{split}\label{eq:mu_flow_equal_r_flow}
\end{align}

Thus, $r_{lt}$ satisfies the flow balance constraint in \eqref{eq:r_flow}. Next, we show that this routing will not exceed any tunnel reservation, i.e, $\sum_t r_{lt} \le a_l$. We know that $\forall t, M\vec{U^*_t} = \vec{D_t}$, so $M\sum_t\vec{U^*_t} = \sum_t\vec{D_t} = \vec{D}$, where $\vec{D}$ is the demand vector with all demands. We have shown in \ref{prop:linear_system} that $MU=\vec{D}$ has a unique solution $U^* \in [0,1]^P$, so $\sum_t\vec{U^*_t} = U^* \in [0,1]^P$. Then $\forall l \in T_x(i,j)$, we have $\sum_t r_{lt} = \sum_t a_l\vec{U^*_t}(i,j)=a_lU^*(i,j) \le a_l$.

\textbf{simpler hints of single link failure.}
The following constraints together with \eqref{eq:tunnel_model} will model $YH$ where for every hint $q$, it is active when the associated link $e_q$ fails.

\begin{align}
\begin{split}
& h_q = x_{e_q} \quad \forall q\\
\end{split}\label{eq:hint_model}
\end{align}

%\sgr{Ignore everything below this.}

%If I need to make the segment robust to failures, then, I need some
%reservation on s-1-4 etc. Let rs14,rs24,rs34 be the reservation on those tunnels. Denote rs14+rs24+rs34 as r.

%This reservation is not available on the s-T tunnels that traverse 1,2,3. Then, when 1-T and 2-T fail, the maximum reservation is 
%0.5 - r/3 on the tunnels not involving 4.
%One surviving tunnel 4 will provide (0.5-rs4)/3.
%So, max reservation on tunnels: 2/3 - (r+rs4)/3

%So total reservation is 2/3 - (r+rs4)/3 + b.
%Make rs4=r/3. Then, b=2r/3. 
%This becomes, 2/3  - 4r/9 + 6r/9 => 2/3 + 2r/9 => 2/3 + b/3
% bis at most 1/2, so 2/3 + 1/6, 5/6

%b is at most the sum of the smallest 2 of rs4, rs34,rs24,rs14
%Make them the same. r=3rs4, b=2rs4.
